# Supplementary material for: Finding Multiple Reaction Pathways of Ligand Unbinding
Source: arXiv:1808.08089 ancillary file (2019-06-17)
Supplement: Supplementary file 1 [file sup.pdf]

# Finding Multiple Reaction Pathways of Ligand Unbinding

**Supporting Information**

Jakub Rydzewski[1,*] and Omar Valsson[2]

[1]*Institute of Physics, Faculty of Physics, Astronomy and Informatics, Nicolaus Copernicus University, Grudziadzka 5, 87-100 Torun, Poland*

[2]*Max Planck Institute for Polymer Research, Ackermannweg 10, D-55128 Mainz, Germany*

## CONTENTS

Model of T4 Lysozyme L99A 1

MD Simulations 1

Loss Function 2

Neighborhood for the Loss Function 2

Minimization Procedure 2

Adaptive Biasing to a Loss Function Minimum 3

Parameters 3

Classification of the Reaction Pathways 3

Biased Unbinding Times 3

Software 3

References 3

## MODEL OF T4 LYSOZYME L99A

The introduced method was tested on the T4 lysozyme L99A (T4L) mutant with bound benzene (PDB ID: 4w52 [1]), which is often used as a model system to study ligand unbinding from proteins. Benzene was parametrized using the LigParGen server [2]. The OPLS-AA/L force field [3] was used in all the simulations. The system was solvated by the SPC water [4]. The resulting complex was electrically neutralized by adding 6 CL ions.

## MD SIMULATIONS

The MD simulations were run using Gromacs-5.1.3 [5]. The system was minimized using the steepest descent algorithm, and then equilibrated through a 10-ns simulation in the NVT ensemble and a 10-ns simulation in the NPT ensemble using the Parrinello-Rahman barostat [6] (1 bar) and the stochastic velocity-rescaling thermostat [7] with benzene and T4L coupled (300 K). A 2-fs time step was used. Periodic boundary conditions and particle mesh Ewald [8] for long-range electrostatics were employed. For short-range interactions a 9 Å cut-off was used. All bond

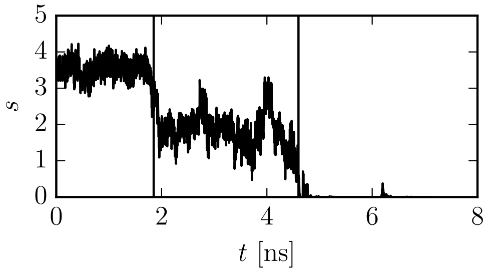


FIG. S1. Loss function along an example trajectory of benzene unbinding from T4L. Two sudden jumps in the loss function indicate conformational transitions of the benzene-T4L complex during unbinding. The first transition at about $t = 1.85$ ns is the change from the bound conformation to an intermediate, during which benzene samples the exit along pwa via D/F/G. Next, at about $t = 4.6$ ns the complex switches its state to unbound.

were constrained using LINCS [9]. Production runs were simulated in the NVT ensemble using the above parameters. In total, 300 10-ns long trajectories were sampled to calculate the reaction pathways of the benzene unbinding from T4L.

## LOSS FUNCTION

To render the loss function unitless, we rescaled the distances between ligand-protein atom pairs applying the length scale $\lambda = 1$ Å$^{-1}$. This also made the loss function invariant with respect to the chosen length units. The protein-ligand atom pairs were found by using a neighbor list between the protein and the ligand, which was recomputed every 0.5 ps with a cut-off for the distance between ligand-protein atom pairs of 7 Å (the cut-off should be larger than the maximal sampling radius). Depending on the current neighborhood of the ligand, the number of protein-ligand atom pairs $P_l$ was not constant, as was the loss function value during the simulations. Using the above scheme of recomputing the loss function at different neighborhoods of the ligand, we were able to find multiple local loss function minima which served as the intermediates of the benzene unbinding through T4L.

## NEIGHBORHOOD FOR THE LOSS FUNCTION

To minimize the loss function, a definition of the neighborhood for the loss function must be provided to find a local minimum. To this end, the loss function is sampled within a sphere centered on the ligand position, and of radius equal to the sampling radius which is computed during the MD simulations as the minimal distance from a ligand atom to a protein atom on the neighbor list. This sphere is an approximation of the conformational space accessible for ligand dissociation, and it is recomputed when the ligand center-of-mass position changes during the simulations.

## MINIMIZATION PROCEDURE

The minimization protocol for the non-convex optimization problem as ligand unbinding was performed using simulated annealing, but any technique suitable for such problem should be sufficient. The initial value of the temperature-like parameter in simulated annealing $T_0$ was 300, and $k$ was set to 0.95 to promote faster convergence to a minimum by limiting the acceptance probability of worse solutions. We used the geometric cooling scheme, i.e., $T$ was modified as $T_j = kT_{j-1}$, where $j$ is the iteration number in the optimization scheme. The cooling factor $k < 1$ is often taken as $> 0.9$, depending on the number of iterations performed to find an optimum. We found that taking

the above parameters and the number of iterations equal to 1000, the optimization scheme was able to reach plateau at the end of the optimization, indicating that no better solution in the ligand neighborhood existed.

## ADAPTIVE BIASING TO A LOSS FUNCTION MINIMUM

Before identifying the biasing rate $v = 0.02$ Å/ps, which was used in all the production runs, at about 140 test simulations were run with biasing rates ranging from 0.02 Å/ps to 1 Å/ps. The force constant $\alpha = 3.6$ kcal/(mol Å) was taken to fit into the so-called stiff-spring regime to ensure that the biasing proceeds with a constant velocity. The direction of biasing (i.e., the loss function minimum) was recalculated every 200 ps, which was enough time for the ligand to change its neighborhood, and thus, the loss function value.

## PARAMETERS

The parameters used in the optimization procedure are not sensitive, and therefore can be transfered to other ligand-protein systems. This is due the locality of the optimized conformational space. The only parameters that need to be chosen before the production runs are the biasing rate and the minimization interval at which the optimization is launched. Typically, the minimization interval should be selected such that the number of possible changes in the unbinding directions during an MD simulation be from 10 to 20, depending on the complexity if the sampled protein tunnels.

## CLASSIFICATION OF THE REACTION PATHWAYS

The unbinding trajectories (300 10-ns simulations) were classified into the five reaction pathways (pwa-e) by inspecting near which protein helices benzene dissociated to solvent (see Fig. 2 in and Tab. 1 the main text for details). The same classification method was employed in Ref. 10. The low standard deviations of the sampling radius and the unbinding time (Tab. 1) for the classified trajectories suggest that benzene dissociated similarly within a given reaction pathway.

## BIASED UNBINDING TIMES

The biased unbinding times were defined as the simulation MD time required for ligand dissociation to reach the loss function value $< 0.1$, which indicated that the ligands exited to solvent. A bootstrapping procedure (1000 sets, each of the sets containing 100% of the trajectories chosen randomly with replacements) was employed to compute the unbinding time distribution for each set of trajectories classified as the same reaction pathway, and to estimate the interim dissociation time as the mean of the distribution and its standard deviation (see Fig. S2).

## SOFTWARE

The method for searching multiple reaction pathways of ligand unbinding is implemented in the official version of the Plumed-2.5 plugin [11], using the C++11 programming language. The implementation is described in Ref. 12.

---

* To whom the correspondence should be addressed: jr@fizyka.umk.pl

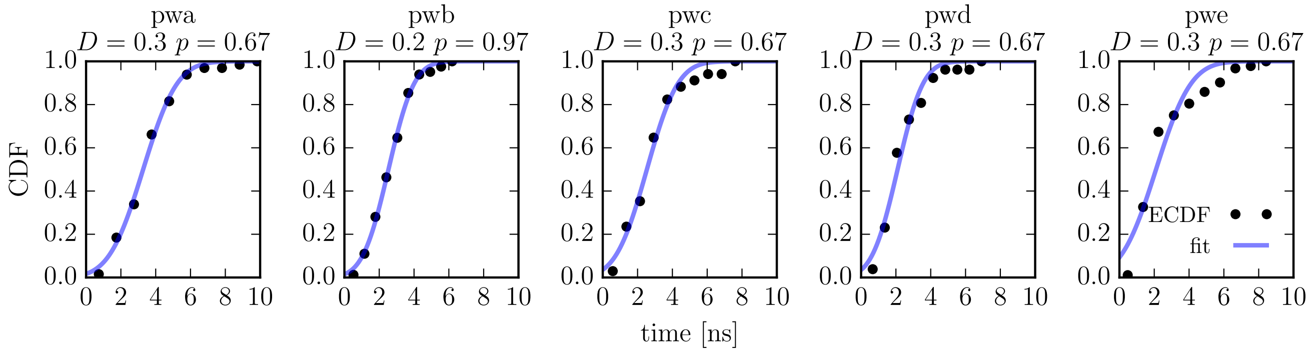


FIG. S2. Analysis of the unbinding time distribution obtained from the biased simulations. The Poisson cumulative distribution function (CDF; $f(t) = 1 - \exp(t/\tau)$) is compared with the empirical cumulative distribution function (ECDF) obtained from the unbinding probability distribution (i.e., the histogram of the number of unbinding events observed in the biased simulations over time) from trajectories for each unbinding pathway. ECDF is shown by black circles, and CDF is depicted by a blue line. $\tau$ values were computed by fitting CDF to the ECDF data. The results of a Kolmogorov-Smirnov (KS) test are quantified by a distance $D$ between fit and ECDF. Typical p-values from KS statistics which quantify the similarity between the empirical and theoretical distributions are also denoted for dissociation times of each pathway.

[1] M. Merski, M. Fischer, T. E. Balius, O. Eidam, and B. K. Shoichet, Proc. Natl. Acad. Sci. U.S.A. **112**, 5039 (2015).
[2] L. S. Dodda, I. Cabeza de Vaca, J. Tirado-Rives, and W. L. Jorgensen, Nucleic Acids Res. **45**, W331 (2017).
[3] G. A. Kaminski, R. A. Friesner, J. Tirado-Rives, and W. L. Jorgensen, J. Phys. Chem. B **105**, 6474 (2001).
[4] Y. Wu, H. L. Tepper, and G. A. Voth, J. Chem. Phys. **124**, 024503 (2006).
[5] M. J. Abraham, T. Murtola, R. Schulz, S. Páll, J. C. Smith, B. Hess, and E. Lindahl, SoftwareX **1**, 19 (2015).
[6] R. Martoňák, A. Laio, and M. Parrinello, Phys. Rev. Lett. **90**, 075503 (2003).
[7] G. Bussi, D. Donadio, and M. Parrinello, J. Chem. Phys. **126**, 014101 (2007).
[8] T. Darden, D. York, and L. Pedersen, J. Chem. Phys. **98**, 10089 (1993).
[9] B. Hess, H. Bekker, H. J. Berendsen, J. G. Fraaije, *et al.*, J. Comput. Chem. **18**, 1463 (1997).
[10] A. Nunes-Alves, D. M. Zuckerman, and G. M. Arantes, Biophys. J. **114**, 1058 (2018).
[11] G. A. Tribello, M. Bonomi, D. Branduardi, C. Camilloni, and G. Bussi, Comput. Phys. Commun. **185**, 604 (2014).
[12] J. Rydzewski, arXiv preprint arXiv:1904.03929 (2019).
